# Supplementary material for: Encouraging Paragraph Embeddings to Remember Sentence Identity Improves Classification
Source: arXiv:1906.03656 source file (2019-06-09)
Supplement: Supplementary file 1 [file supplemental.tex]

Supplemental Material
